# Supplementary material for: AGNNCert: Defending Graph Neural Networks against Arbitrary Perturbations with Deterministic Certification
Source: arXiv:2502.00765 source file (2025-02-02)
Supplement: Supplementary file 1 [file appendix_old.tex]

\section*{Appendix}


\begin{table*}[!t]
\label{tbl:notations}
%\begin{wraptable}{r}{0.6\textwidth}
    \footnotesize
    \centering 
    %\scriptsize
    %\tiny
    \renewcommand\arraystretch{1.3}
    \begin{tabular}{c|c|c|c|c|c|c|c}
     \toprule
    Graph&$G$&Nodes&$\mathcal{V}$&Edges&$\mathcal{E}$&Node features&$\mathbf{X}$\\
    \cline{1-8} 
    Node/Graph classifier&$f$&Neighborhood&$\mathcal{N}$&Layer Number&$L$&hidden features&$\mathbf{h}^{l}$\\
    \cline{1-8} 
    Layer Weight&$\mathbf{W}^{l}$&Scale Function&$\alpha$&Active Function&$\sigma$&Robust Classifier&$\overline{f}$\\
    \cline{1-8}
    Node Label&$y_{v}$&Node Classification&$f(G)_{v}$&Graph Label&$y_{G}$&Graph Classification&$f(G)$\\
    \cline{1-8}
    Node Vote&$c_{y_{v}}$&Graph Vote&$c_{y_{G}}$&Vote Node Classification&$\overline{f}(G)_{v}$&Vote Graph Classification&$\overline{f}(G)$\\
    \cline{1-8}
    Perturbed Graph&$G'$&Perturbed Node&$\mathcal{V}'$&Perturbed Edge&$\mathcal{E}'$&Perturbed Feature&$\mathbf{X}'$\\
    \cline{1-8}
    Class Set&$\mathcal{Y}$&Injected Edge&$\mathcal{E}_{+}$&Deleted Edge&$\mathcal{E}_{-}$&Injected Node&$\mathcal{V}_{+}$\\
    \cline{1-8}
    $\mathcal{V}_{+}$ Associated Edge&$\mathcal{E}_{\mathcal{V}_{+}}$&$\mathcal{V}_{+}$ Features&$\mathbf{X}_{{V}_{+}}$&Deleted Node&$\mathcal{V}_{-}$&$\mathcal{V}_{-}$ Associated Edge&$\mathcal{E}_{\mathcal{V}_{-}}$\\
    \cline{1-8} 
    $\mathcal{V}_{-}$ Features&$\mathbf{X}_{{V}_{-}}$&Feature Manipulated Node&$\mathcal{V}_{r}$&$\mathcal{V}_{r}$ Associated Edge&$\mathcal{E}_{\mathcal{V}_{-}}$&$\mathcal{V}_{r}$ Features&$\mathbf{E}_{\mathcal{V}_{r}}$\\
    \cline{1-8}
    $\mathcal{V}_{r}$ New Features&$\mathbf{X}_{\mathcal{V}_{r}}'$&Subgraph Amount&$T$&Subgraphs&$\mathcal{G}_{T}$&Perturbed Subgraphs &$\mathcal{G}'_{T}$\\
    \cline{1-8}
    Hash Function&$h$&Edge's Subgraph Index&$\hat{i}_{e}$&Subgraph&$G_{i}$&Edges in $G_{i}$&$\hat{\mathcal{E}}_{i}$\\
    \cline{1-8}
    String Function& str()&Certified Bound&$M$\\
 \bottomrule
    \end{tabular}
        \caption{Summary of the important notations used in the paper.}
    \label{tbl:notations}
    %\vspace{-4mm}
%\end{wraptable}
\end{table*}



\subsection{Proof of Theorem~\ref{thm:suffcond}}

\begin{proof}
\begin{equation}
    \mathbf{V}_{y_{a}}-\mathbb{I}(y_{a}>y_{b})\geq \mathbf{V}_{y_{b}}
\end{equation}
\begin{equation}
    \mathbf{V}_{y_{b}}-\mathbb{I}(y_{b}>y_{c})\geq \mathbf{V}_{y_{c}}, \forall y_c \in \mathcal{Y}\setminus\{y_{a}\}
\end{equation}
We note the attacked votes of the class $y_a$ and any other class $y_{c}\in \mathcal{Y}\setminus \{y_{a}\}$:
\begin{equation}
\mathbf{V}_{y_{a}}'\geq \mathbf{V}_{y_{a}} - \sum_{i=1}^{T}\mathbb{I}(f(G_{i})_v\neq f(G'_{i})_v) 
\end{equation}
\begin{equation}
\mathbf{V}_{y_{c}}'\leq \mathbf{V}_{y_{c}} + \sum_{i=1}^{T}\mathbb{I}(f(G_{i})_v\neq f(G'_{i})_v)
%\leq \mathbf{V}_{y_{b}}-\mathbb{I}(y_{b}>y_{c}) + \sum_{i=1}^{T}\mathbb{I}(f(G_{i})_v
\end{equation}
To ensure the vote prediction not changed, it needs to satisfy:
\begin{equation}
\mathbf{V}_{y_{a}}'\geq \mathbf{V}_{y_c}'+\mathbb{I}(y_{a}>y_{c}),\forall y_{c}\in \mathcal{Y}\setminus \{y_{a}\}
\end{equation}
A sufficient condition for this equation could be obtained by applying eq(24-25):

\begin{equation}
\mathbf{V}_{y_{a}}\geq \mathbf{V}_{y_{c}} + 2\sum_{i=1}^{T}\mathbb{I}(f(G_{i})_v\neq f(G'_{i})_v)+\mathbb{I}(y_{a}>y_{c})
\end{equation}
%We also give a certified bound $M$ and a attack evaluation function $e(S)$ for any arbitrary attack with size features $S$ targeting the general-robust problem in eqn(\ref{eqn:fullyrobust}). These will be discussed in Section~\ref{Sec:Certification}.
Applying the eqn(22), we further relax this condition as:
\begin{equation}
\mathbf{V}_{y_{a}} \geq \mathbf{V}_{y_{b}}-\mathbb{I}(y_{b}>y_{c})+ 2\sum_{i=1}^{T}\mathbb{I}(f(G_{i})_v\neq f(G'_{i})_v)+\mathbb{I}(y_{a}>y_{c})
\end{equation}
We observe that:
\begin{equation}
\mathbb{I}(y_{a}>y_{b})\geq \mathbb{I}(y_{a}>y_{c})-\mathbb{I}(y_{b}>y_{c})
,\forall y_{c}\in \mathcal{Y}\setminus \{y_{a}\}\end{equation}
Therefore, a final sufficient condition for eqn(26) is:
\begin{equation}
\mathbf{V}_{y_{a}} \geq \mathbf{V}_{y_{b}}+2\sum_{i=1}^{T}\mathbb{I}(f(G_{i})_v\neq f(G'_{i})_v)+\mathbb{I}(y_{a}>y_{b})
\end{equation}
which is equivalent as eqn(23).
\label{Sec:VotingClass}
\end{proof}


\subsection{Proofs of Theorem \ref{thm:edgeperturb}-\ref{thm:nodefeaperturb}}
\label{proof:edgepart}
First we prove Theorem \ref{thm:edgeperturb}, which is straightforward:
\begin{proof}(For Theorem \ref{thm:edgeperturb})
    
\end{proof}

To prove theorem \ref{thm:nodeperturb}-\ref{thm:nodefeaperturb}, (1) we first introduce the theorem \ref{thm:isolatedinedge}, which illustrates that: in every edge-cerntric subgraph, any manipulation on isolated nodes or their features have no influence on the predictions; (2) then we prove that after the node or feature manipulation, there are only a few amount of subgraphs where the perturbed nodes are not isolated, while in others they are all isolated and therefore the predictions maintain.

\begin{theorem}
\label{thm:isolatedinedge}
For a subgraph $G_{i}=\{\mathcal{V},\mathbf{X}, \mathcal{E}_{i}\}$, if an isolated node $u$ (not the target node $v$) with feature $\mathbf{X}_{u}$ from $G$:
\begin{enumerate}
    \item is deleted:
    $G_{i}' = \{\mathcal{V}\setminus\{u\},  \mathbf{X}\setminus \mathbf{X}_{u},  \mathcal{E}_{i}\}$
    \item is injected: $G_{i}' = \{\mathcal{V}\cup\{u\},  \mathbf{X}\cup \mathbf{X}_{u},  \mathcal{E}_{i}\}$
    \item whose feature is perturbed with arbitrary feature $\mathbf{X}'_{u} :G_{i}' = \{\mathcal{V},  \mathbf{X}\setminus\mathbf{X}_{u}\cup \mathbf{X}'_{u},  \mathcal{E}_{i}\}$
\end{enumerate}
the prediction on $G'_i$ does not change, i.e., $f(G_i) = f(G'_i)$. 
%on the attacked subgraph $f(G_{i}')$ is still the same with $f(G_{i})$.
\end{theorem}
\begin{proof}
For every other node $w\in\mathcal{V}\setminus\{u\}$, its $0$-layer hidden $\mathbf{h}_{w}^{0}$ is the same after attack:
\begin{equation}
    \mathbf{h}_{w}^{0'}=\mathbf{h}_{w}^{0} = \mathbf{X}_{w}
\end{equation}
Since $u$ is an isolated node, $w$'s neighborhood $\mathcal{N}(w)$ is the same after attack:
\begin{equation}
    \mathcal{N}(w)' = \mathcal{N}(w)
\end{equation}
For every message passing layer $l$ defined in eqn(\ref{eqn:Message}), we observe if the neighborhood $\mathcal{N}(w)$ and the $(l-1)$-th hiddens for $w$ and $\mathcal{N}(w)$ are the same after attack, then the $l$-th hidden for $v$ is the same as well:

\begin{equation}
\begin{aligned}
    &(\mathbf{h}^{l-1}(\mathcal{N}(w)) = \mathbf{h}^{'l-1}(\mathcal{N}(w)))\wedge(\mathbf{h}^{l-1}(w) = \mathbf{h}^{'l-1}(w))\\
    &\wedge (\mathcal{N}(w)' = \mathcal{N}(v))\Rightarrow \mathbf{h}^{'l}(w) =\mathbf{h}^{l}(w)
\end{aligned}
\end{equation}
Combined with eqn(17), we could deductively prove the final hidden $\mathbf{h}^{L}$ is the same for every node $w$:
\begin{equation}
 \mathbf{h}^{'L}_{w} = \mathbf{h}^{L}_{w}, \forall w \in \mathcal{V}\setminus\{u\}
\end{equation}
For the node classification on the target node $v\in \mathcal{V}\setminus\{u\}$, the prediction result is the same since its hidden is the same; for the graph classification, since $u$ is isolated, it will be deleted initially, and the subgraph will remain the same together with its prediction.
\end{proof}
Then utilizing Theorem \ref{thm:isolatedinedge}, we prove the Theorem \ref{thm:nodeperturb} and \ref{thm:nodeperturb}:
\begin{proof}(For Theorem \ref{thm:nodeperturb})
 For node manipulation, in $T$ Edge-Centric subgraphs, edges connected to injected nodes $\mathcal{E}_{\mathcal{V}_+}$ will be mapped to at most $|\mathcal{E}_{\mathcal{V}_+}|$ subgraphs after injection, and edges deleted with nodes $\mathcal{E}_{\mathcal{V}_+}$ exist in at most $|\mathcal{E}_{\mathcal{V}_-}|$ subgraphs before the deletion. Therefore there are at least $T-(|\mathcal{E}_{\mathcal{V}_+}|+|\mathcal{E}_{\mathcal{V}_-}|)$ subgraphs where these deleted nodes and injected nodes are all isolated. According to Theorem~\ref{thm:isolatedinedge}, predictions on these $T-(|\mathcal{E}_{\mathcal{V}_+}|+|\mathcal{E}_{\mathcal{V}_-}|)$ subgraphs will not change after the manipulations. In other words, there are at most $|\mathcal{E}_{\mathcal{V}_+}|+|\mathcal{E}_{\mathcal{V}_-}|$ subgraphs would give different predictions. 
\end{proof}
\begin{proof}(For Theorem \ref{thm:nodefeaperturb})
 For feature manipulation, in $T$ Edge-Centric subgraphs, edges connected to representative nodes $\mathcal{E}_{\mathcal{V}_r}$ exist in at most $|\mathcal{E}_{\mathcal{V}_r}|$ subgraphs. Therefore there are at least $T-|\mathcal{E}_{\mathcal{V}_r}|$ subgraphs where these representative nodes are all isolated. According to Theorem~\ref{thm:isolatedinedge}, predictions on these $T-|\mathcal{E}_{\mathcal{V}_r}|$ subgraphs will not change after the manipulations. In other words, there are at most $|\mathcal{E}_{\mathcal{V}_r}$ subgraphs would give different predictions. 
\end{proof}

% \begin{theorem}[]
% \label{thm:nodeperturb}
% If the original graph is injected with $\{\mathcal{V}_{+}, {\bf X}_{\mathcal{V}_+}, \mathcal{E}_{\mathcal{V}_+}\}$, or deleted with $\{\mathcal{V}_{-}, {\bf X}_{\mathcal{V}_-}, \mathcal{E}_{\mathcal{V}_-}\}$, or replaced on feature with $\{\mathcal{V}_{r}, {\bf X}_{\mathcal{V}_{r}}, \mathcal{E}_{\mathcal{V}_{r}}\}$, there are at most $|\mathcal{E}_{\mathcal{V}_+}|$/$|\mathcal{E}_{\mathcal{V}_-}|$/$|\mathcal{E}_{\mathcal{V}_{r}}|$ subgraphs would give different predictions from the original ones.
% \end{theorem}
% \begin{proof}
%  For node addition, in $T$ Edge-Centric subgraphs, edges $\mathcal{E}_{\mathcal{V}_+}$ will be mapped to at most $|\mathcal{E}_{\mathcal{V}_+}|$. Therefore there are at least $T-|\mathcal{E}_{\mathcal{V}_+}|$ subgraphs where these injected nodes are all isolated. According to Theorem~\ref{thm:isolatedinedge}, predictions on these $T-|\mathcal{E}_{\mathcal{V}_+}|$ subgraphs will not change, and therefore there are at most $|\mathcal{E}_{\mathcal{V}_+}|$ subgraphs would give different predictions. This proof is the same for node deletion and the feature attack.
% \end{proof}


\subsection{Proofs of Theorem~\ref{thm:edgeperturb2}-\ref{thm:nodefeaperturb2}}
\label{proof:nodepart}
%We observe that our Node-Centric subgraphs have the 
\begin{theorem}%[Subgraphs Similarity]
%[Bounded Number of Different Subgraphs]
\label{thm:embUnchange}
For a subgraph $G_{i}=\{\mathcal{V},{\bf X},\mathcal{E}_{i}\}$, assume a node $u\in \mathcal{V}$ with node feature ${\bf X}_{u}$ only having incoming edge $\mathcal{E}_{u}$ in $\mathcal{E}$. If $u$:
\begin{enumerate}
\item is deleted:  $G_{i}=\{\mathcal{V}\setminus\{u\},{\bf X}\setminus\mathbf{X}_{u},\mathcal{E}_{i}\}$
%\vspace{-2mm} 
\item $u$ gets polluted on features $X_{u}$; 
%\vspace{-2mm} 
\item a new node $u'$ is injected into $\mathcal{V}$ with arbitrary directed edges targeting $u'$ injected into $\mathcal{E}$;
\end{enumerate}
the node embedding on original nodes $\{h^{\circ}_{v},\forall v\in \mathcal{V}\setminus\{u\}\}$ will always stay the same  in any above case.
%\vspace{-2mm} 
\end{theorem}
\emph{Proof.} According to the definition of neighborhood we made in eqn(\ref{eqn:neighborhood}), the neighborhoods of other nodes in $\mathcal{V}\setminus\{u\}$ remain the same after above cases:
$$\mathcal{N}'(v) = \mathcal{N}(v), \forall v \in \mathcal{V}\setminus\{u\}$$
Then under the message passing functions described in eqn(\ref{eqn:GCNMessage}-\ref{eqn:GATMessage}) with trained weights, since $u$ (or $u'$) never appears in any other nodes' neighborhood, the hidden features in every layer are calculated the same:
$$\mathbf{h}_{v}^{l}{}' = \mathbf{h}_{v}^{l}, \forall v \in \mathcal{V}\setminus\{u\}, l \in [1,L]$$
and the final node embeddings stay the same as well. 
